# Supplementary material for: A single-shot measurement of time-dependent diffusion over sub-millisecond timescales using static field gradient NMR
Source: arXiv:2012.12968 ancillary file (2021-03-03)
Supplement: Supplementary file 1 [file Supplementary_Material.pdf]

# Supplementary Material:
# A single-shot measurement of time-dependent diffusion over sub-millisecond timescales using static field gradient NMR

**CONTENTS**


**I Python code to generate $m_j$** . . . . . . . . . . 2

**II MATLAB code** . . . . . . . . . . 4

A Monte Carlo simulations

B LLS inversion

C Fitting procedures

**III Echo time dependence of results** . . . . . . . . . . 12

**IV Supplementary methodology** . . . . . . . . . . 13

A NMR experimental methods

B SG-TIETA pulse program

C Complete echo shape characterization

D Relaxation time measurements

**References** . . . . . . . . . . 14

## I. PYTHON CODE TO GENERATE $m_j$

Python (3.7) code to generate $m_j$ sequences given $\tau$ and $\delta$ is provided here. The spacing sequence, $\{\tau, 2\tau + m_1\delta, ..., 2\tau + m_j\delta\}$ can be treated as a list of integers when converted to whole number microseconds. Helper functions, provided below, were written to check satisfaction of individual rules.

For rule (ii) – "$m_j$ and $m_{j\pm\Delta j}$ with odd $\Delta j$ may not be the same." – duplicates, or "dupes" in the spacing sequence were found and then iteratively checked for an odd index difference. Rule (ii) addresses $\Sigma\Delta F(t)$ with two terms.

```
from numpy      import diff
from itertools  import combinations, intersection

def findDupes(seq):
    # finds and returns entries with at least one duplicate in a list
    seen = set()
    dupes = list()
    for x in seq:
        if x not in seen:
            seen.add(x)
        else:
            if x not in dupes:
                dupes.append(x)
    return(dupes)

def checkDupes(seq):
    # check rule (ii)
    dupes = findDupes(seq)
    if not dupes:                                               # no duplicates found
        return True
    else:
        for dupe in dupes:
            ind = [i for i, x in enumerate(seq) if x == dupe]
            # list indices with a duplicate
            diff_indices = diff(ind)
            diff_even = list(map(lambda x: x%2, diff_indices))
            # check even/odd index difference
            if 1 in diff_even:                                  # at least 1 odd
                break
            elif dupe == dupes[-1]:                             # last unique duplicate
                return True                                     # pass
        return False                                            # fail
```

Rule (iii) – "Twice any $m_j$ may not equal the sum of $m_{j+\Delta j}$ and $m_{j-\Delta j}$ for even $\Delta j$." – was checked by pulling all possible ordered "triples" in the spacing sequence, iterating through odd $\Delta j$, or "sep", in the outer loop and the central index in the inner loop. Rule (iii) addresses $\Sigma\Delta F(t)$ with three terms.

```
def checkTriples(seq):
    # check rule (iii)
    found = False                                               # flag
    for sep in range(1, (len(seq) - 1)//2 + 1, 2):
    # iterate through odd index separations
        for i in range(sep, len(seq) - sep):
        # iterate through possible center indices
            triple = (seq[i - sep], seq[i], seq[i + sep])
            if sum([triple[0], triple[1]*-2, triple[2]]) == 0:  # found off-resonance CTP
                found = True                                    # change flag and exit
                break
        if found: break                                         # inner -> outer break
    return not found
```

Rules (iv–v) – “Any two $m_j$ with even $j$ may not equal the sum of any two $m_j$ with odd $j$.” and “Twice any $m_j$ with even $j$ may not equal the sum of any two $m_j$ with odd $j$, and vice versa.” – were addressed by taking all even and odd entries' indices in the spacing sequence and leveraging `itertools` dependencies to find all unique even and odd sums and their intersections. Anything present in the intersections constitutes a rule violation. Rules (iv–v) address $\Sigma\Delta F(t)$ with four terms.

```
def checkQuadruples(seq):
    # check rules (iv) and (v)
    odds = seq[0::2]                                            # odd entries in sequence
    odd_sums = set(map(sum, list(combinations(delay_odds, 2)))) # find all unique odd pair sums
    evens = seq[1::2]
    even_sums = set(map(sum, list(combinations(delay_evens, 2))))
    return not (odd_sums.intersection(even_sums) or \                   # rule (iv)
                odd_sums.intersection(evens*2)   or \                   # rule (v)
                even_sums.intersection(odds*2))                         # rule (v) vice versa
```

Rules were next checked in aggregate. Rule (i) – “Absolute $F(t)$ heights, or $h_n$, may not be repeated.” – was addressed by calculating and storing heights. Repeated height entries were disallowed. Additional restrictions were incorporated. Echoes were forced to form, i.e., the $F(t)$ height must change sign after each $\pi$-pulse. Also, no height is allowed to be less than $\gamma g\tau$ to prevent the formation of echoes with very little diffusion attenuation. Selection of $\tau$ therefore also specified the minimum useful $b$-value.

```
def checkDelaySeq(seq):
    # check all rules + practical rules for echo formation and minimum F(t) height
    seen = list()                                    # store the seen heights
    ht_curr = seq[0]                                 # first height is tau (divided by gamG)
    seen.append(ht_curr)
    for i in range(1, len(seq)):
        ht_next = ht_curr + (-1)**(i%2)*delay_seq[i] # recursive height definition, Fig. 2
        if (ht_curr*ht_next > 0)    or \             # sign change = echo formation
           (abs(ht_next) in seen)   or \             # rule (i)
           (abs(ht_next) < seq[0]):                  # minimum height and therefore b
            return False
        else:
            seen.append(abs(ht_next))
        ht_curr = ht_next
    return(checkDupes(seq)   and \                   # satisfies all rules
           checkTriples(seq) and \
           checkQuadruples(seq))
```

Finally, $m_j$ was found iteratively. For each new entry in $m_j$, values were tried, starting from 1, until $m_j$ is valid according to the above function(s). The $m_j$ list was first converted to a spacing sequence. Console output of $m_j$ up to 100 terms using the timing parameters in Eq. (15) is shown. The code as provided is efficient enough to find sequences of arbitrary useful length, i.e. up to hundreds of echoes. Further time/space complexity optimization may be possible but is superfluous. Future work might involve developing analytical equations for pulse spacing optimizations, similar to the the optimized spacing for decoupling of spin coherence from the presence of noise presented by Uhrig[1].

```
tau = 49                 # microseconds
delta = 14               # chosen to follow rule (vi), 49 (mod 14) = 7 = 14/2
curr_m_j = [1, 3]        # seed sequence
final_len = 100          # number of echoes/delays
max_m = 3*final_len      # ensure loop break at some max guess

def convertSeq(m_j, tau, delta):
    # convert m_j to spacings
```

```
    seq = list()
    seq.append(tau)
    seq.extend([x*delta+2*tau for x in var])
    return delay_seq

try_m_j = list()
while (len(curr_m_j) < final_len) and (m < max_m):
    # simple implementation: iteratively find sequence that works, naively prefer small m_j
    try_m_j = curr_m_j
    try_seq.append(m)
    if checkDelaySeq(convertSeq(try_seq, tau, delta)):
        curr_m_j = try_m_j
        m = 1
    else:
        m += 1

print(curr_seq)
Out[1]:
[  1   3   6   7  10  12  11  15  20  21  24  26  20  21  33  35  33  34
  33  39  47  44  42  44  47  53  56  53  52  58  61  67  70  67  65  67
  75  85  88  85  79  76  88  90  79  85  93  90  97 103 102 103 111 108
 102 117 120 122 120 117 120 117 120 117 120 131 139 140 134 140 143 140
 148 158 157 149 143 145 157 167 175 168 157 163 175 177 166 163 175 181
 189 195 189 181 175 181 189 195 203 209]
```

## II. MATLAB CODE

In this section, we provide representative code (MATLAB 2019A, Mathworks, Natick, MA) and commentary for the (A) Monte Carlo simulations, (B) the LLS inversion, and (C) the various fitting procedures described in the text.

### A. Monte Carlo simulations

Simulations were performed using an off-the-shelf MATLAB tool: "MCSD: A MATLAB Tool for Monte-Carlo Simulations of Diffusion in Biological Tissues"[2] (https://github.com/davidnsousa/mcsd). The tool is used to create geometries of permeable and impermeable parallel cylinders. These parameters were used throughout:

```
D = 2.15E-9;
t = 700E-6;          % simulate up to 700 microseconds
t_steps = 700;       % 1 microsecond steps
n_walkers = 25000;
dt = t/t_steps;
l = 12E-6;                              % arrange cylinders in a 12x12 micron region
initial_position = rand(3, n_walkers)*l; % places walkers in cube/box
step_size = sqrt(6*D*dt);               % distance step size
```

The geometry of the barriers was created using the `cells()` function, which randomly places non-overlapping cylinders into a specified square region. The parameters were then passed to `rwalk()` which performs the random walk simulation. The trajectories of the first 100 walkers for each geometry are shown in Fig. S1 below. Geometries are described in the code and the figure caption. The $\langle[\mathbf{r}(t)\cdot\hat{\mathbf{g}}]^2\rangle$ curves shown in Fig. 3a were taken from the $y$-direction here, i.e., orthogonal to the cylinders. The black (circles), free diffusion curve was taken from the $z$-direction of the red (triangles) curve. To generate the smoothed gradient curves in Fig. 3c, local gradient points were averaged and smoothed using a moving average filter with a span of 0.1.

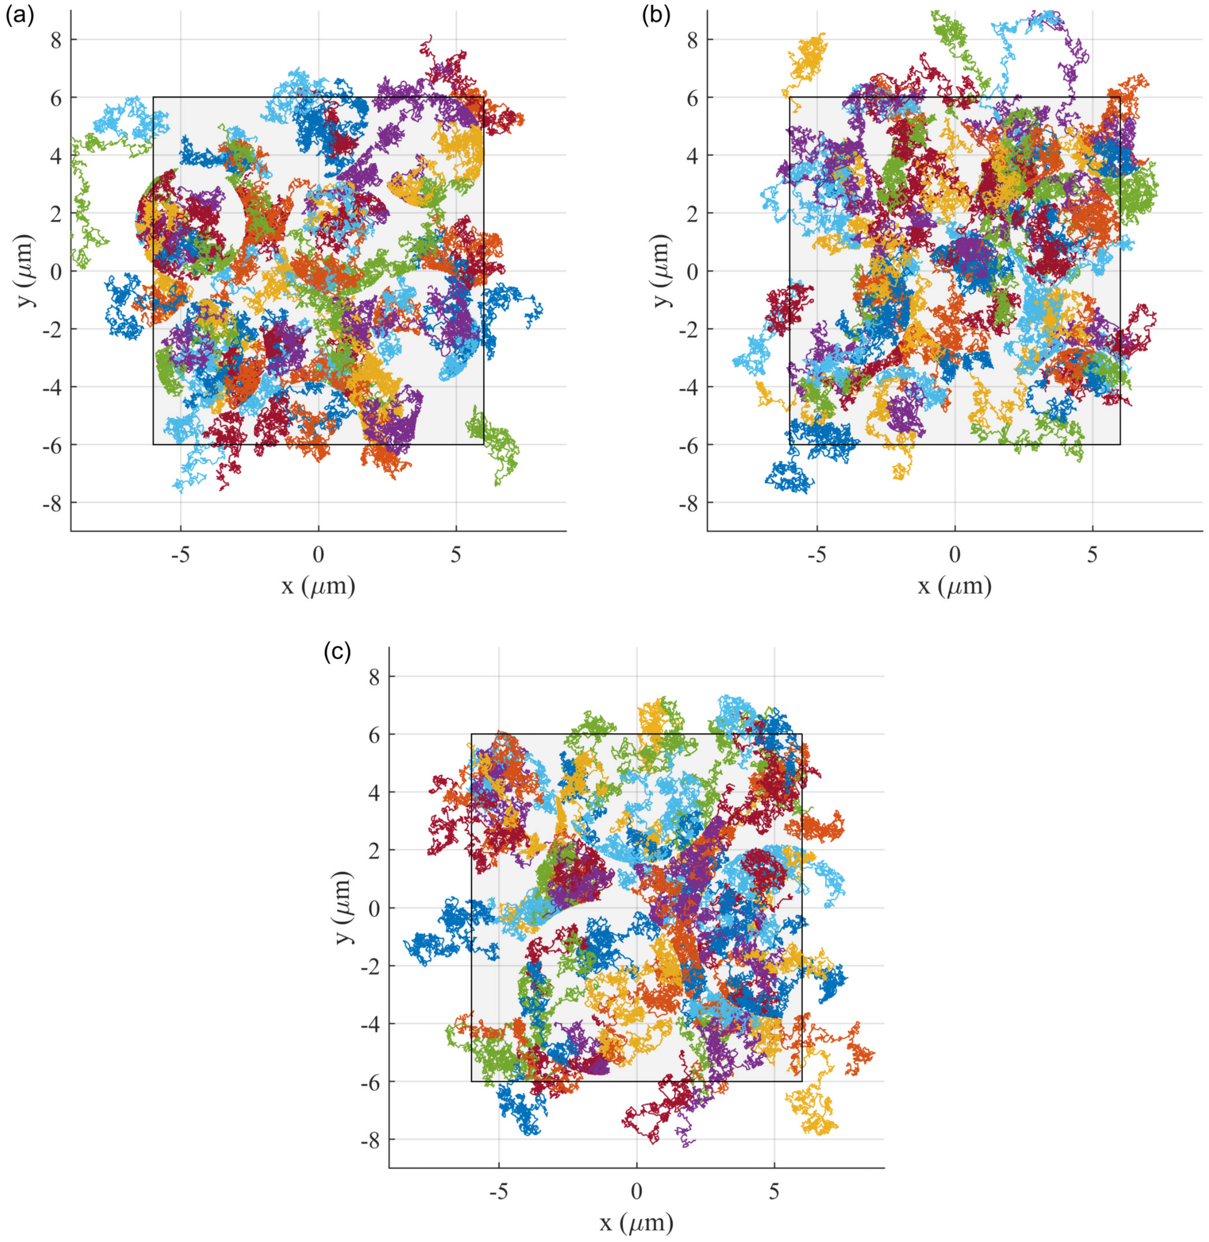


FIG. S1. Sample Monte Carlo simulation trajectories for $\langle [\mathbf{r}(t) \cdot \mathbf{g}]^2 \rangle$ curves presented in Fig. 3 of the main text. (a) Trajectories for blue curve: eight non-overlapping impermeable cylinders ($R = 1$ $\mu$m) with faces randomly packed into a $12 \times 12$ $\mu$m box, traced in black. All walkers start from random positions within the box. (b) Trajectories for red curve: same configuration as (a) but with 4% cross-over probability upon cylinder wall collision. (c) Trajectories for magenta curve: four impermeable cylinders ($R = 1.5$ $\mu$m) in the same box.

```
% blue curve in Fig. 3; 8x 2 micron diameter cylinders
C = cells(ones(8,1)*2E-6, [0 1 0 1]);
geometry = @(x,y,z) C(x,y);
X = rwalk(initial_position, t_steps, step_size, geometry) % run simulution

% red curve in Fig. 3
% same configuration as previous,
% w/permeability corresponding to 4% cross-over probability on collision
C = cells(ones(8,1)*2E-6, [0 1 0 1]);
geometry = @(x,y,z) C(x,y);
permeability = 4E-2;
```

```
X = rwalk(initial_position, t_steps, step_size, geometry, permeability);

% magenta curve in Fig. 3; 4x 3 micron diameter cylinders
C = cells(ones(4,1)*3E-6, [0 l 0 l]);
geometry = @(x,y,z) C(x,y);
X = rwalk(initial_position, t_steps, step_size, geometry)

% to make MSD curves as in Fig. 3a
MSD_y = mean(transpose(X(:,:,2) - X(1,:,2)).^2);
MSD_z = mean(transpose(X(:,:,3) - X(1,:,3)).^2);

% to make gradient curves as in Fig. 3c
span = 0.1;
Dinst_y = gradient(smooth(MSD_y, span)/(dt*2));
Dinst_z = gradient(smooth(MSD_z, span)/(dt*2));

% to plot 100 sample trajectories centered at (0,0)
X_scaled = X(:,:,:).*1E6;
plot3((X_scaled(:,1:100,1)-l/2*1E6),...
      (X_scaled(:,1:100,2)-l/2*1E6),...
      (X_scaled(:,1:100,3)-l/2*1E6));
view(0,90)
```

## B. LLS inversion

To perform the LLS inversion in Figs. 3 and 6, **W**, **B**, **A**, and initial **X** guesses were specified. Pulse sequence parameters define **A**. A function was written to find the timings and heights from a given $m_j, \tau$, and $\delta$. The code follows from the caption of Fig. 2.

```
function [t, T] = calcTimings(m_j, tau, del)
    % given SG-TIETA m_j, delta, tau, return the times of pulses and echoes
    spacings = [tau (2*tau+del.*m_j)];

    function [abs_hts] = calculateHt(spacings)
        % helper fxn to find heights
        abs_hts = zeros(1, length(spacings));
        abs_hts(1) = spacings(1);
        for i = 2:length(m_j)
            abs_hts(i) = abs(spacing(i) - abs_hts(i-1));    % see Fig. 2 caption
        end
    end

    abs_hts = calculateHt(spacings);
    t = [0 cumsum(spacings)];
    T = [0 (t(2:end)+abs_hts)];                          % see Fig. 2a, magenta line
end
```

$C_n(t)$ piecewise symbolic curves were generated using the timings given in Eq. (15). $b$-values were also calculated.

```
tau = 49E-6; % Eq. (15)
del = 14E-6;
m_j = [ 1 3 6 7 10 12 11 15 20 21 24 26 20 21 33 35 33 34 33];
%m_j = [ 1 3 6 7 10 12 11 15 20 21 24 26 20 21 33 35 33 34 33 ...
%        39 47 44 42 44 47 53 52 58 61 67 70 67 65 67 75 85 88 85 79]; % longer m_j for D6
                                                                       % results in Fig. 6
N = length(m_j) + 1;
```

```
D0 = 2.15E-9;
gamma2g2 = 16.6837E18; % from G = 15.3 T/m

[t_n, T_n] = calcTimings(m_j, tau, del);
h_n = diff(T_n)./2;
C_n = sym(zeros(N, 1));

syms t
for i = 1:N
    C_n(i) = gamma2g2*...       % solution given in Eq. (14)
        piecewise(...
            0<=t<=h_n(i),        t*(2*h_n(i)-3*t/2), ...
            h_n(i)<=t<=2*h_n(i), t*(-2*h_n(i)+t/2)+2*h_n(i)^2, ...
            2*h_n(i)<=t,         0);
end
b = 2/3*gamma2g2.*cumsum(h_n.^3);
```

**A** can be calculated by integrating over $C_n(t)$ given $\Delta t(k)$. For all data other than the D6 data, $\Delta t(k)$ was chosen to be $\{50, 50, 50, 50, 75, 75, 125, 183\}$ $\mu$s which gives $t$ integration bounds of

$$\sum_k \Delta t(k) = \{0, 50, 100, 150, 200, 275, 350, 475, 658\} \ \mu\text{s}.$$

For D6, the range is extended to (see code above)

$$\Delta t(k) = \{50, 50, 50, 50, 75, 75, 125, 125, 125, 125, 150, 200\} \ \mu\text{s},$$

which gives $t$ bounds of

$$\sum_k \Delta t(k) = \{0, 50, 100, 150, 200, 275, 350, 475, 600, 725, 850, 1000, 1200\} \ \mu\text{s}.$$

```
function [A] = calcA(C_n)
    % definition of A given in Eq. (13)
    t_bounds = csvread('t_bounds.csv'); % read in t bounds described above
    A = zeros(length(C_n), length(t_bounds) - 2);
    for i = 1:length(C_n)
        C = C_n(i);
        for j = 1:length(t_bounds)-1
            A(i, j) = int(C, [t_bounds(j) t_bounds(j+1)]);
        end
    end
end
```

With **A** in hand, simulated data was generated by calculating the echo attenuation from the smoothed gradient curves discussed in the previous section, i.e., curves were numerically integrated from $t = 0$ to $T$ according to Eq. (10). Gaussian noise was then added to the resulting $I(T)/I_0$ curves (Fig. 3b) over 100 noise replications. Finally, decays were converted to the log ratio form of **B** for the LLS inversion shown in Fig. 3c.

```
function [atten] = calcAttenuation(t, Dinst, C)
   % calculate attenuation for a given echo interval and C_n
   prod = zeros(length(t), 1);      % store product of C_n and D_inst
   for i = 1:length(t)
       t_val = t(i);
       C_val = subs(C, t_val);      % substitute t
       prod(i) = C_val*Dinst(i);
   end
   atten = exp(-trapz(t, prod));    % numerically integrate the product, i.e., Eq. (10)
end
```

```
function [I] = calcI(t, Dinst, C_n)
    % calculate normalized echo intensity, I(T), curves from C_n, D_inst, and t array
    attens = ones(length(C_n), 1);
    for n = 1:length(C_n)
        attens(n) = calcAttenuation(t, Dinst, C_n(n)); % calculate inter-echo attenuations
    end
    I = cumprod(attens);                              % cumulative product = I(T)/I_0
end

% example call, t_lim = rightmost t bound
I_ya = [1; calcI(0:dt:t_lim, Dinst_ya, C_n)] % blue curve in Fig. 3

% generate simulated data
N_min = 3;  % exclude first 2 echo ratios, see Fig. 3
N_max = 20; % stop at N = 20
A = A(N_min:N_max,:);

SNR = 25;
n_reps = 100;
seed = 1234;
I_no_noise = [I_ya I_yb I_yc I_zc];             % a,b,c,d correspond to -->
                                                % (Fig. 3) blue, red, magenta, black
I_sim = repmat(I_no_noise, [1 1 n_reps]);       % allocate simulated data repetitions
W = zeros(size(I_sim,1)-1, size(I_sim,2));      % allocate weights matrix
for n = 1:n_reps
    rng(seed,'twister');
    noise = randn(size(I_no_noise))*(1/SNR)^2;  % Gaussian noise with variance of 1/SNR^2
    I_sim(:,:,n) = I_sim(:,:,n) + noise;        % additive noise
    W(:,:,n) = abs(min(diff(I_sim(:,:,n)),0));  % weights = difference, removing negative terms
    seed = seed + 1;
end
B_sim = -log(I_sim(N_min+1:N_max+1,:,:)./I_sim(N_min:N_max,:,:)); % B = log echo ratios
```

$\mathbf{\Gamma}$ consisted of a concatenation of forward first-order ($\mathbf{L}_1$) and differently spaced central second-order finite difference matrices ($\mathbf{L}_2$ and $\mathbf{L}_3$),

$$\mathbf{L}_1 = \begin{bmatrix} 1 & -1 & & \\ & \ddots & \ddots & \\ & & 1 & -1 \end{bmatrix}, \; \mathbf{L}_2 = \begin{bmatrix} 1 & -2 & 1 & & \\ & \ddots & \ddots & \ddots & \\ & & 1 & -2 & 1 \end{bmatrix}, \\ \mathbf{L}_3 \begin{bmatrix} 2 & 0 & -4 & 0 & 2 & & \\ & \ddots & \ddots & \ddots & \ddots & \ddots & \\ & & 2 & 0 & -4 & 0 & 2 \end{bmatrix}, \; \mathbf{\Gamma} = \begin{bmatrix} \mathbf{L}_1 \\ \mathbf{L}_2 \\ \mathbf{L}_3 \end{bmatrix}. \tag{S1}$$

$\mathbf{\Gamma}$ was created based on the dimensions of $\mathbf{A}$. $\lambda$ was manually selected as $2 \times 10^{-6}$. $D_0$ and approximated $D_\infty$ values were used for initial $\mathbf{X}$ guesses as described in Fig. 3. The LLS inversion was performed using the `lsqr()` function, which is an adaptation of the conjugate gradients method for rectangular matrices.

```
function L = calcL(A)
    % definition given in Eq. (S1)
    L_1 = zeros(size(A,2)-1, size(A,2));
    for i = 1:size(L_1,1)
        L_1(i,i) = 1;
        L_1(i,i+1) = -1;
    end
    L_2 = zeros(size(A,2)-4, size(A,2));
    for i = 1:size(L_2,1)
        L_2(i,i) = 2;
```

```
        L_2(i,i+2) = -4;
        L_2(i,i+4) = 2;
    end
    L_3 = zeros(size(A,2)-2, size(A,2));
    for i = 1:size(L_3,1)
        L_3(i,i) = 1;
        L_3(i,i+1) = -2;
        L_3(i,i+2) = 1;
    end
    L = [L_1; L_2; L_3];
end

L = calcL(A);
lambda = 2E-6;

% perform LLS inversion
solns = zeros(size(A,2), size(B_sim,2), size(B_sim,3)); % allocate solns
Dinf = [0.9E-9 1.45E-9 1.48E-9 2.15E-9];
for n = 1:n_reps
    for i = 1:size(B_sim,2)
        wts = (repmat(W(N_min:end, i, n), 1, size(I_sim,1))).^0.5;  % W^(1/2)
        solns(:,i,n) = lsqr([wts*A; lambda*L],...
        % concatenate norm and reg term
                                    [wts*I_sim(:,i,n); zeros(size(L,1), 1)],...
                                   0.25E-15, 1000, [], [], [D0; ones(size(A,2)-1,1).*Dinf(i)]);
                                   % initial guess = D_0 first point, D_inf for remaining points
    end
end
```

The LLS procedure was exactly the same for experimental data shown in Fig. 6, except that no echo ratios are discarded and a pre-processing (fitting) step was performed beforehand, discussed in the text and in the following SM subsection. Note that this LLS inversion is highly sensitive to the initial guess due to the comparative lack of sensitivity at the tails of $D_{\text{inst}}(t)$, as demonstrated below in Fig. S2. Accurate prior knowledge of $D_0$, $D_\infty$, and $A_p(n)$ is necessary.

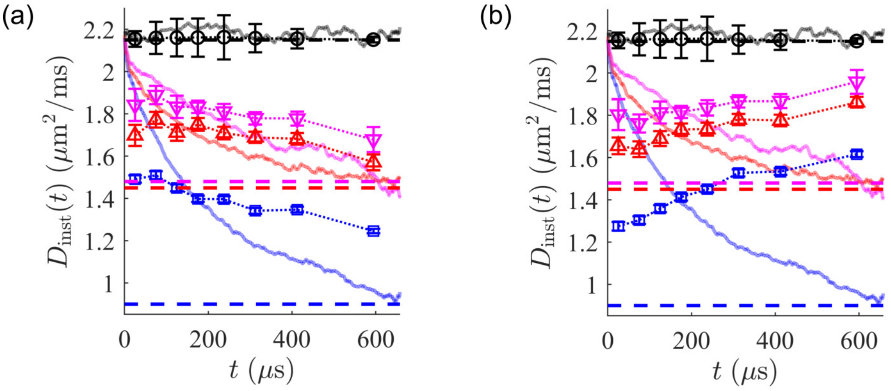


FIG. S2. Demonstration of LLS inversion sensitivity to initial guess. (a) Inversion result if the initial guess is a flat line at $D_\infty = \{0.9, 1.45, 1.48\}$ $\mu$m$^2$/ms. (b) Inversion result if the initial guess is a flat line at $D_0$.

## C. Fitting procedures

All fitting was performed with another off-the-shelf MATLAB tool: “SLM - Shape Language Modeling”[3], which conveniently allows for the specification of conditions such as upwards concavity in a (piece-wise linear or cubic) least squares fit. For the pulse accuracy fitting, data was acquired in the form of 32× summed, 16 $\mu$s echo windows per repetition. Example decay data for 1-octanol are shown

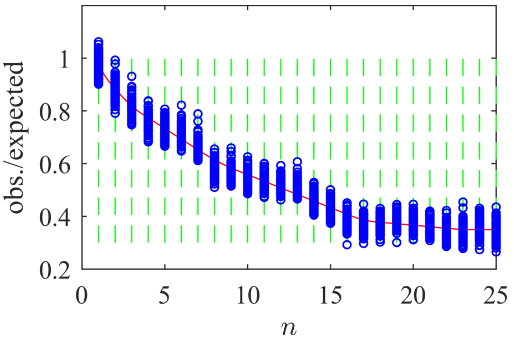


FIG. S3. Piece-wise cubic fitting of 1-octanol data described in Fig. 4b and performed in the code below. Expected decay is given by $\exp(-bD_0)$ using $D_0$ values obtained from spin echo diffusion experiments described in SM Section IV. Points are shown from all 70 repetitions. Green, dashed lines demarcate $n$. The obtained fit is shown in red.

below. Data was normalized to the first echo. The expected decay (see Fig. 4a) was calculated using the $b$-values obtained previously. A piecewise cubic fit (see Fig. 4b) was then performed to the observation vs. expected decay in the $n$-domain, specified to be decreasing, concave up, and weighted by the signal intensity. $A_p(n)$ values were then determined using adjacent ratios of the fitted curve values. Fig. S3 demonstrates the 1-octanol fitting. The same procedure was used for the water and decane data.

---

```
% Example octanol data for several repetitions, note the 32x summing
%{
n = 1       n = 2       ...
31.43       30.79       27.25       24.97       23.67       22.31       22.13       20.82
30.53       30.09       27.44       25.00       23.23       22.28       21.87       20.27
29.57       29.84       27.96       25.45       23.23       21.89       21.86       20.56
31.04       28.61       27.23       25.76       22.72       22.52       20.61       20.71
30.15       30.26       28.07       26.77       23.13       23.06       21.49       20.36
30.95       30.48       27.47       25.23       24.17       22.10       22.02       20.05
31.21       29.24       27.46       25.18       23.11       23.23       23.82       20.91
31.24       28.73       27.75       25.12       22.57       22.99       23.19       20.57
%}

D_octanol = 1.2116E-10;                          % D0 measured by spin echo diffusion, Sec. IV
I_octanol = csvread('octanol_16.csv');           % raw data, e.g. above
I_octanol = I_octanol./I_octanol(:,1);           % normalize to first echo
I_octanol = I_octanol(:,2:end);                  % remove first echo
I_octanol_th = exp(-D_octanol*(b(2:end)-b(1))); % expected decay

n_octanol = 25;
obs_ratio_octanol = I_octanol(:,1:n_octanol)./I_octanol_th(:,1:n_octanol);
% obs./expected ratio
n_vals_octanol = transpose(kron(1:n_octanol, ...
                           ones(size(obs_ratio_octanol,1),1)));
                           % reshape ratio data for fit
n_vals_octanol = reshape(n_vals_octanol.',1,[]);
wts_vals_octanol = kron(sqrt(mean(I_octanol(:,1:n_octanol))),...
% weights for fit = mean signal
                        ones(size(obs_ratio_octanol,1),1));
obs_ratio_octanol_forslm = reshape(obs_ratio_octanol, 1, []);
slm_octanol = slmengine(n_vals_octanol, obs_ratio_octanol_forslm, ...   % slm fit
                'decreasing', 'on',...
                'maxvalue', 1,...
                'deg', 3,...            % cubic
                'concaveup', 'on',...
                'knots', n_octanol,...  % n-1 cubic "pieces"
```

```
                'weights', wts_vals_octanol);
obs_ratio_octanol_slm = slmeval(1:n_octanol, slm_octanol);
% evaluate fit at n
Ap_octanol_slm = obs_ratio_octanol_slm(2:end)./obs_ratio_octanol_slm(1:end-1);
% obtained A_p values
```

For the $b$-domain fitting of yeast and D6 data, a similar procedure was used. Decays were again normalized to the first echo. Decays were then corrected with the pulse accuracy curves obtained in Fig. 4c. A piecewise linear fit was then performed, specified as described in the text. Fig. S4 demonstrates fitting for one of the yeast curves and for the D6 curve. The LLS inversion was then performed as described in the previous section. Exemplar code for one of the yeast datasets is shown below.

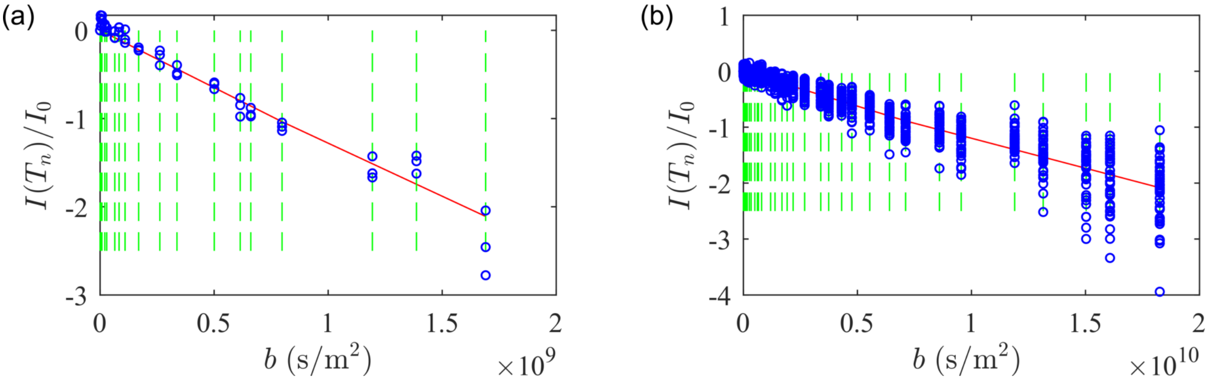


FIG. S4. Monotone derivative piece-wise log-linear fitting between adjacent $b$-values, as described in the text. (a) Fit for lower density yeast (2.84B cells/mL). Green, dashed lines demarcate $b$-values which serve as fit interval bounds. All 3 repetitions are shown. (b) Fit for D6. All 38 repetitions are shown.

```
D0 = 2.22E-9;
acc = csvread('pulse_acc.csv', 1, 0);    % A_p(n)
acc = cumprod(acc);

I_yeast1 = csvread('yeast1_16.csv');
I_yeast1 = I_yeast1./I_yeast1(:,1);      % normalize
I_yeast1 = I_yeast1(:,2:end);

n_yeast1 = 17;  % truncate at this echo
I_yeast1_acc = horzcat(ones(size(I_yeast1,1),1),...
% concat 1's for b = 0
                       I_yeast1(:,1:n_yeast1)./acc(1:length(I_yeast1_mean))); % correct A_p(n)
I_yeast1_acc = reshape(I_yeast1_acc, 1, []);                                   % reshape data
b_yeast1 = kron([0 b(1:n_yeast1)], ones(size(I_yeast1_acc,1),1));              % b-values
wts_slm_yeast1 = sqrt(kron([1 I_yeast1_mean], ones(size(I_yeast1_acc,1),1))); % weights

slm_yeast1 = slmengine(b_yeast1, log(I_yeast1_acc), ...
                'decreasing', 'on',...
                'concaveup', 'on',...                 % i.e., slopes monotonically decrease
                'leftvalue', 0, ...                   % leftmost point
                'maxslope', D0,...                    % max slope of D0
                'degree', 1,...
                'knots', unique(b_yeast1),...         % fit between all adjacent b-values
                'weights', wts_slm_yeast1);
I_yeast1_slm = exp(slmeval(b(1:n_yeast1), slm_yeast1));

B_yeast1 = -log(I_yeast1_slm./[1 I_yeast1_slm(1:end-1)]);   % log echo ratio for fit
I_yeast1_slm_diff = abs(diff([1 I_yeast1_slm]));            % signal difference = weights
wts_yeast1 = repmat(I_yeast1_slm_diff, length(I_yeast1_slm_diff ), 1).^0.5; % W^(1/2)
```

```
A_yeast1 = A(2:n_yeast1+1,:);    % skip first row because of normalization
L_yeast1 = computeL(A_yeast1);

Dinf_yeast1 = 0.9E-9;
soln_yeast1 = lsqr([wts_yeast1*A_yeast1; lambda*L_yeast1],...
                [wts_yeast1*B_yeast1.'; zeros(size(L_yeast1, 1), 1)],...
                0.25E-15, 1000, [], [], [D0; ones(size(A_yeast1,2)-1,1).*Dinf_yeast1]);
```

## III. ECHO TIME DEPENDENCE OF RESULTS

In order to assess both the validity of our pulse accuracy correction and the relative contribution of $T_2$, the analysis in the text was repeated for a different value of $\tau = 77$ $\mu$s ($\delta = 14$ $\mu$s, and same $m_j$). This $\tau$ still satisfies rule (vi). A longer $\tau$ contains more $T_2$ and diffusion weighting.

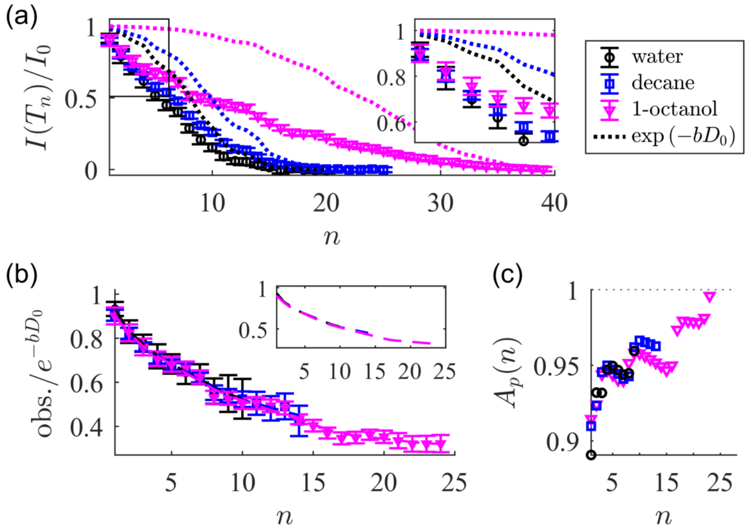


FIG. S5. Pulse accuracy analysis in Fig. 5 repeated using data obtained for $\tau = 77$ $\mu$s. Expected decay is given by $\exp(-bD_0)$ using $D_0$ values obtained with spin echo diffusion experiments described in SM Section IV. Repetition numbers are, in legend order: 25, 38, 70. Error bars = ± 1 SD.

In Fig. S5, similar results are obtained for the pulse accuracy analysis compared to Fig. 4c, providing strong preliminary support for our conception of $A_p(n)$ as being only $n$-dependent, irrespective of diffusion weighting. We acknowledge, however, that $A_p(n)$ remains incompletely understood. The origin of the jaggedness seen across all liquids, for example, is unclear. Future work may clarify the causes of this observed $A_p(n)$ behavior. Using the same $A_p(n)$ obtained for water in the main text, SG-TIETA yeast decays using this longer $\tau$ were collected and analyzed. Results are shown below in Fig. S6.

Expectedly, these yeast decays and resulting $\mathbf{X}$ values are similar in magnitude to the results in Fig. 6. Here, however, the confounding effects of $T_2$ relaxation are more apparent. Longer intervals exhibit larger than expected decay and shorter intervals exhibit comparatively smaller decay. The short-time behavior of both yeast curves is less separated compared to the main text, perhaps due to the higher yeast density having a shorter measured $T_2$ (see SM Section IV.D). Thus, while $T_2$ was ignored in the main text on the basis of $(2\tau + m_j\delta) \ll T_2\ \forall j$, $T_2$ may affect the presented results, as illustrated by the $\tau$-dependent changes in inverted $\mathbf{X}$ behavior. Yeast $D_{\mathrm{inst}}(t)$ results in the main text thus fall short of quantitative accuracy due to $T_2$ contributions and other factors presented in the discussion.

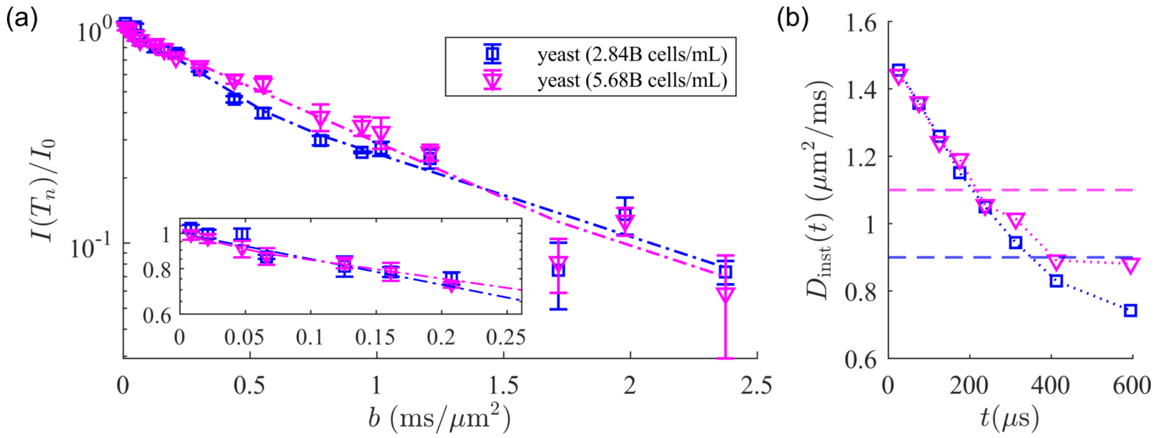


FIG. S6. Yeast results using $\tau = 77$ $\mu$s. (a) Signal decay normalized to the first echo and fit as described in the text and the previous section. Decays are truncated at $n = 17$. Error bars = $\pm$ 1 SD. (b) Inverted $\mathbf{X}$ values using $\Delta t(k) = \{50, 50, 50, 50, 75, 75, 125, 183\}$ $\mu$s, an adjusted $\mathbf{A}$, and the same inversion parameters ($\mathbf{\Gamma}$, $\mathbf{W}^{1/2}$, $\lambda = 2 \times 10^{-6}$).

## IV. SUPPLEMENTARY METHODOLOGY

### A. NMR experimental methods

Experimental protocols involved looping through SG-TIETA experiments, spin echo diffusion experiments, and CPMG experiments to acquire repetitions of each experiment. Noise and probe tuning was monitored at the beginning of each loop and was seen to be stable for all samples.

SG-TIETA experiments were performed at different echo times TE = $2\tau$ = [98, 126, 147, 154, 182, 210, 238, 266, 294, 322, 350, 378, 406, 434, 462, 490] $\mu$s, with 101 echoes, incremental delay of $\delta = 14$ $\mu$s, and using the integer delay list $m_j$ calculated and presented in SM Section I. SG-TIETA experiments use the standard 2-step phase cycle used for CPMG where the phase of the first 90° pulse and the receiver are cycled between $+x$ and $-x$ while the phase of the 180° pulses is kept as $y$. Spin echo diffusion measurements involved a spin echo diffusion encoding block followed by a CPMG acquisition[4] block in which 2000 echoes were acquired with TE = 25 $\mu$s. The $\tau$ of the diffusion encoding block was varied linearly over 22 points from $\tau_{\rm min} = 0.05$ ms to $\tau_{\rm max} = [1, 1, 2.2, 2.2, 2.2]$ for water, decane, 1-octanol, D6, and yeast, respectively. CPMG experiments were performed using 2000 echoes and 96 $\mu$s echo time. For all experiments, the RF pulse length was set to 1.6 $\mu$s, 90°/180° pulse power = -22/-18 dB and the repetition time was set to between 3 and 5$\times$ the $T_1$ of the sample ([10, 5, 2, 2, 2] s for water, decane, 1-octanol, D6, and yeast respectively). Echoes were acquired with dwell time = 0.5 $\mu$s and acquisition window = [16, 4, 16] $\mu$s for SG-TIETA, spin echo diffusion, and CPMG experiments respectively. The real signal from the central 16 of the total 32 pts. of each SG-TIETA echo was summed to represent the echo signal.

### B. SG-TIETA pulse program

A 140 ns delay was added between the first 90° excitation pulse and the first 180° refocusing pulse. This delay was needed to prevent a drift of the echoes, however this drift is not seen with the standard CPMG. The optimal delay value is independent of pulse power. The pulse program was written to include the optimal $m_j$ delay increments generated in SM Section I. Since the list includes 100 increments and no increment is used prior to the first echo, up to 101 echoes can be acquired.

Note that this $m_j$ list is not unique. Other $m_j$ lists optimized for different initial $\tau$ and $\delta$ values were implemented with similar results. The measured diffusion coefficient began to increase when using $\delta < 10$ $\mu$s due to signal from unwanted coherence transfer pathways refocusing near the direct echo. A slightly larger value, $\delta = 14$ $\mu$s, was chosen. This value may need to be optimized depending on the pulse time, as discussed in the text. Larger $\delta$ values can be chosen to probe a larger range of timescales.

Timings in the pulse program are defined differently than in Fig. 2. The delay list used by the pulse program, $m_j^{ppg}$, is defined from the $m_j$ list by $m_j^{ppg} = m_j - m_{j-1}^{ppg}$ with $m_1^{ppg} = 0$.

No significant difference was seen between the attenuation and echo shape of odd and even echoes.

### C. Complete echo shape characterization

For completeness, we have included all individual echo shapes and an exemplar SG-TIETA echo decay to accompany Fig. 5. Fig. S7 contains echo shapes from $n = 1$ to 32 and verifies our statement that the echo shapes stabilize around $n = 3$ – little to no substantive variation in the real echo shape is observed thereafter. Fig. S8 shows a complete echo decay for an exemplar 1-octanol experiment. Off-center variations in the signal may be due to the tails of indirect echoes, i.e., echoes that are associated with the refocusing of off-resonance CTPs.

### D. Relaxation time measurements

$T_1$ relaxation time values were measured for all samples using the standard saturation recovery sequence on the NMR-MOUSE with 21 recovery times spaced logarithmically to a value near $5 \times T_1$. A single exponential model fit well to the data, with $T_1$ values shown in Table I.

The CPMG acquisition from the first $\tau$ of the SEdec experiments was fit with a single exponential model to estimate an apparent, diffusion-weighted $T_2$. The diffusion weighting during the CPMG decay was minimized by using a short TE (= 25 $\mu$s). The obtained $T_2$ values are shown in Table I. The pure fluids show a trend of decreasing $T_2$ with increasing diffusion coefficient. This decrease is due to diffusion weighting.

In order to remove the influence of the gradient, a homogeneous magnet with a similar magnetic field strength was used to measure the $T_2$ relaxation time distribution on a sample of the yeast #2 suspension on the same day that SG-TIETA measurements were performed. A standard CPMG sequence was used on a Pure Devices MagSpec low-field MR instrument ($B_0$ = 0.55 T, $\omega_0$ = 23.5 MHz). 1666 echoes were acquired with with a 300 $\mu$s echo time. A distribution was estimated from the signal decay using a standard non-parametric model with $\ell 2$ regularization. The $T_2$ distribution is shown in Fig. S9. 95% of the $T_2$ distribution has $T_2 \gtrsim 10$ ms while the remaining 5% has $T_2 \approx 500$ $\mu$s. In the SG-TIETA measurement, this $T_2$ is similar to $\max\{2\tau + m_j\delta\} = 539$ $\mu$s. It is expected that $T_2$ weighting associated with this short $T_2$ population will cause the signal to decay slightly faster. For the other 95 % of the signal, the diffusion decay is expected to be separated from the $T_2$ decay. Methods to remove the effects of $T_2$ relaxation will be necessary for the study of more viscous materials with short $T_2$ or for the use of SG-TIETA on magnets with smaller gradient strengths. Future work will involve utilizing an additional magnet with a homogeneous magnetic field and at the same field strength as the NMR-MOUSE in order to correct for the decay due to relaxation.

## REFERENCES


[1] G. S. Uhrig, Phys. Rev. Lett. **98**, 100504 (2007).

[2] D. N. Sousa and H. A. Ferreira, J. Open Source Softw. **3**, 966 (2018).

[3] J. D. D'Errico, *Slm - shape language modeling* (2017), URL `https://www.mathworks.com/matlabcentral/fileexchange/24443-slm-shape-language-modeling`.

[4] D. Rata, F. Casanova, J. Perlo, D. Demco, and B. Blümich, J. Magn. Reson. **180**, 229 (2006).

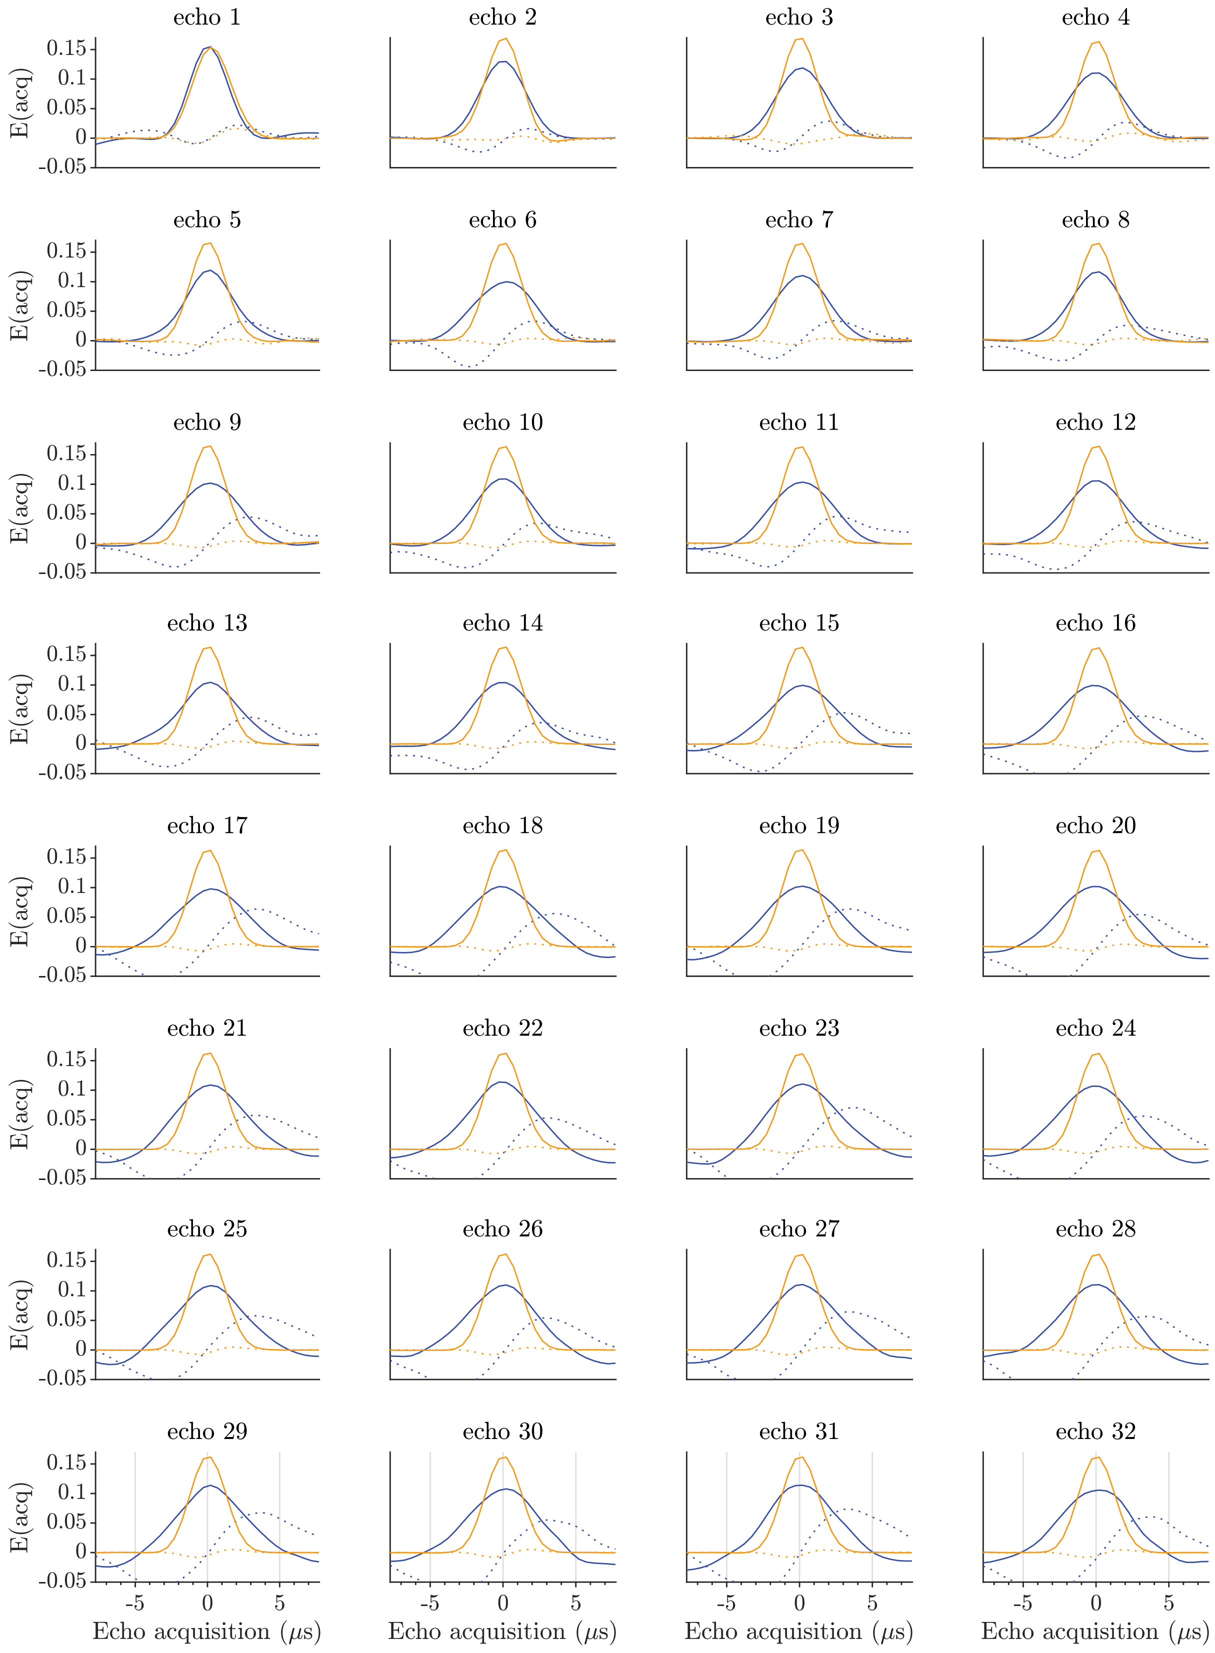


FIG. S7. Comparison of the direct echo SG-TIETA (blue) and CPMG (orange) echo shapes for 1-octanol with $2\tau = \mathrm{TE} = 98$ ms. Echo shapes show the real (solid lines) and imaginary (dotted lines) signal normalized by the area under the real signal curve in a 16 $\mu$s window. As discussed in Fig. 5, the CPMG echo width decreases with $n$, whereas the SG-TIETA echo width increases.

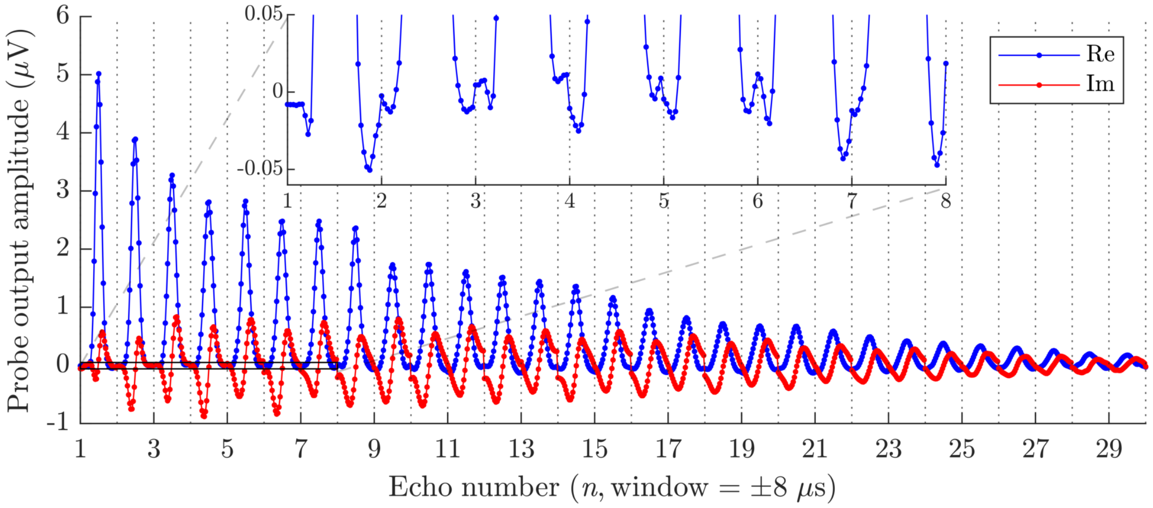


FIG. S8. Exemplar SG-TIETA echo decay for 1-octanol. Real and imaginary signal is shown in raw probe amplitude units. Echoes are stitched together and plotted by echo number, labelled to the left, i.e., the points between $n = 1$ and 2 correspond to the first echo. Zoomed inset shows amplitude variations which may arise from indirect echo contributions.

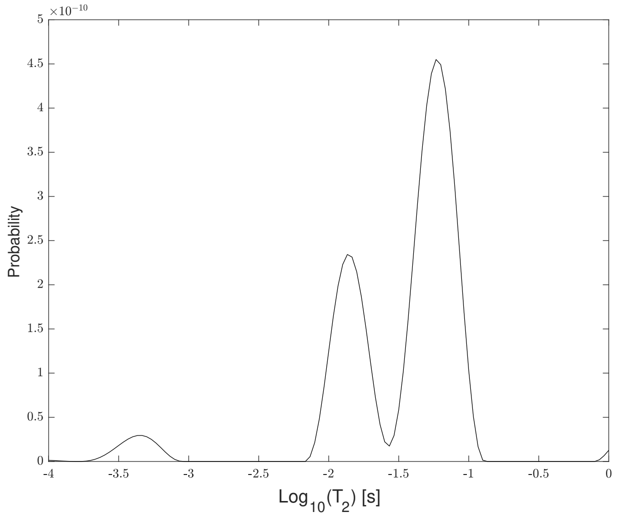


FIG. S9. $T_2$ distribution for the yeast #2 sample measured using a CPMG sequence, echo time = 300 $\mu$s on a homogeneous magnet with $B_0 = 0.55$ T.
